# Supplementary material for: Fluctuating magnetism of Co- and Cu-doped NaFeAs
Source: arXiv:2103.13161 source file (2021-03-24)
Supplement: Supplementary file 1 [file Supplemental_Material_to_Fluctuating_magnetism_of_Co__and_Cu_doped_NaFeAs_v2.pdf]

# Supplemental Material to "Fluctuating magnetism of Co- and Cu-doped NaFeAs"

Jonathan Pelliciari,[1,2,*] Kenji Ishii,[3] Lingyi Xing,[4] Xiancheng Wang,[4] Changqing Jin,[4,5] and Thorsten Schmitt[1,†]

[1]*Photon Science Division, Paul Scherrer Institut, CH-5232 Villigen PSI, Switzerland*

[2]*NSLS-II, Brookhaven National Laboratory, Upton, NY 11973, USA*

[3]*Synchrotron Radiation Research Center, National Institutes for Quantum and Radiological Science and Technology, Sayo, Hyogo 679-5148, Japan*

[4]*Beijing National Lab for Condensed Matter Physics, Institute of Physics, Chinese Academy of Sciences, Beijing 100190, China*

[5]*Collaborative Innovation Center for Quantum Matters, Beijing, China*

## I. SAMPLE PREPARATIONS

The single crystals of $NaFe_{1-x}Co_xAs$ and $NaFe_{1-x}Cu_xAs$ have been grown by the self-flux method, using NaAs as flux. The precursor, $Na_3As$, has been prepared by mixing Na lumps and an As powder, which had been sealed in an evacuated titanium tube and sintered at 650° C for 10 h. The other precursor, $Fe_{1-x}Co_xAs$ ($Fe_{1-x}Cu_xAs$), has been synthesized by mixing Fe, Co, (Cu,) and As powders, which has been compressed into pellets, and sealed in an evacuated quartz tube. After this, a sintering phase at 700° C for 20 h has been performed. The complete homogeneity of the samples has been achieved by further grounding and sintering the pellets. The stoichiometric amount of $Na_3As$, $Fe_{1-x}Co_xAs$ ($Fe_{1-x}Cu_xAs$), and As powder has been weighted according to the element ratio to achieve $Na(Fe_{1-x}Co_x)_{0.3}As$ ($Na(Fe_{1-x}Cu_x)_{0.3}As$). The mixture has been grounded and put into an alumina crucible and sealed in a Nb crucible under 1 atm of argon gas. The Nb crucible has been sealed in an evacuated quartz tube and heated to 900° C before being slowly cooled down to 600° C (3° C/h) to grow single crystals. All sample preparations, except for sealing, has been carried out in a glove box filled with high-purity argon gas. The elemental composition of the $NaFe_{1-x}Co_xAs$ and $NaFe_{1-x}Cu_xAs$ single crystals has been controlled by energy-dispersive x-ray spectroscopy (EDS). Samples have been finally stored in a sealed quartz tube and prepared for spectroscopic studies in a glove box under high-purity $N_2$ flow to avoid contact with air.

We measured samples of $NaFe_{1-x}Co_xAs$ of x = 0.03 optimally doped with $T_C$ = 20 K and x = 0.08 overdoped with $T_C$ = 6 K and $NaFe_{1-x}Cu_xAs$ x = 0.02 optimally doped with $T_C$ = 12 K and x = 0.03 overdoped with $T_C$ = 5 K.

### A. Fe-K edge XAS and XES

Fe-K edge XAS and XES experiments have been carried out at BL11XU of SPring-8, Hyogo, Japan. The incoming photon beam has been monochromatized by a Si[111] double-crystal and a Si[400] secondary channel-cut crystal. The energy has been calibrated through the measurement of x-ray absorption of a polycrystalline Fe foil. As a spectrometer, we have employed three spherical diced Ge[620] analyzers and a detector in Rowland geometry at about 2 m distance from the analyzers. The total combined resolution has been tuned

to about 400 meV, estimated from the FWHM of the elastic line. XAS at the Fe-K edge has been measured in partial fluorescence yield (PFY) mode setting the analyzer to 7.059 keV and scanning the incident energy from 7.10 keV up to 7.15 keV. The intensity has been normalized by the incident flux monitored by an ionization chamber. XAS-PFY spectra have all been collected at 15 K. The energy of the incident x-rays of the XES experiments has been set to 7.140 keV with $\pi$ polarization, and the outgoing photon energy scanned between 7.02 keV and 7.08 keV. The intensity has been normalized similarly to the XAS by the incident flux which is monitored by an ionization chamber. XES spectra have been recorded at 15 and 300 K employing a closed cycle He cryostat.

The samples have been mounted on a sample holder inside a glove box under high-purity He flow and then enclosed in a capsule with a Be window to avoid air contamination.

### B. Integrated Absolute Difference (IAD)

To establish the values of $\mu_{bare}$ we used the integrated area difference (IAD)[1]. We first calculated the center of mass for all the spectra and aligned the spectra along the energy axis as described in Ref. 2 to correct for possible energy misalignment. We normalized the XES spectra areas to the same values, then we calculated the difference with the reference spectrum of FeCrAs which has been used as a calibrating material in other studies[1–6]. The integral of the difference spectrum gives the IAD, which is directly proportional to $\mu_{bare}$[1]. We set the IAD value for $BaFe_2As_2$ to 1.00 to compare with the literature.

In Fig. 1, we show the difference spectra between the parent and the overdoped samples for the Co (a) and Cu (b) doping cases. For the Co cases we observe a difference in the difference spectrum recorded as a green filled area. This indicates a change of $\mu_{bare}$ in the overdoped compound as summarized in Fig. 4 of the main text. Looking into Fig.1, we observe very little difference between the Cu overoped case and NaFeAs which points to an independence of $\mu_{bare}$ from doping.

In Fig.2, we show the raw data of $NaFe_{1-x}Co_xAs$ and $NaFe_{1-x}Cu_xAs$ at 300 K as black line and FeCrAs (reference) as red line. In the bottom panels we display the difference spectra from where the IAD is obtained. To highlight the change of $\mu_{bare}$ as a function of temperature we report in Fig. 3 the difference between the spectra of NaFeAs, Cu-, and Co-overdoped compounds at 15 and 300K. We can clearly see the presence of a peak in the

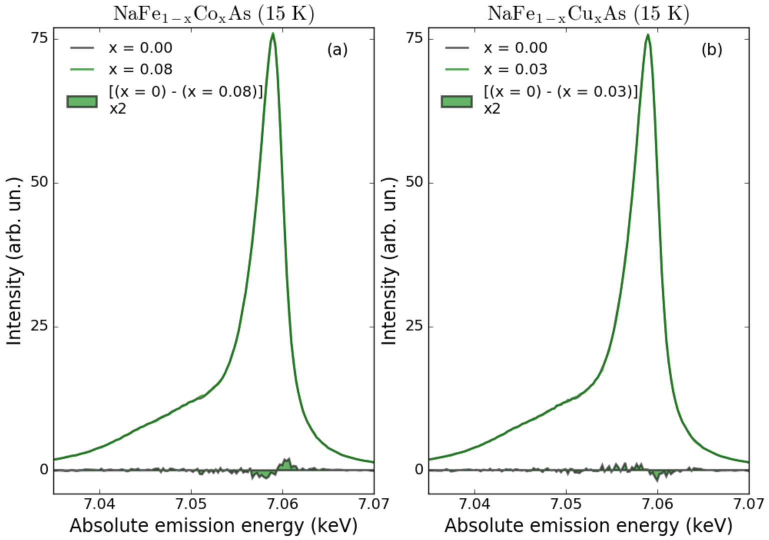


FIG. 1. XES spectra of NaFeAs, $NaFe_{1-x}Co_xAs$ x= 0.08 (a), and $NaFe_{1-x}Cu_xAs$ x= 0.03 (b). We also show the difference between XES spectra of the two overdoped samples and NaFeAs at 15 K.

difference spectrum (red filled area) which indicates the change of $\mu_{bare}$ as summarized in Fig. 4 of the main text.

* pelliciari@bnl.gov

† thorsten.schmitt@psi.ch

[1] G. Vank, T. Neisius, G. Molnr, F. Renz, S. Krpti, A. Shukla, and F. M. F. de Groot, The Journal of Physical Chemistry B **110**, 11647 (2006).

[2] P. Glatzel and U. Bergmann, Coordination Chemistry Reviews Synchrotron Radiation in Inorganic and Bioinorganic Chemistry, **249**, 65 (2005).

[3] K. Tsutsumi, H. Nakamori, and K. Ichikawa, Physical Review B **13**, 929 (1976).

[4] U. Bergmann and P. Glatzel, Photosynthesis Research **102**, 255 (2009).

[5] G. Vank, A. Bordage, P. Glatzel, E. Gallo, M. Rovezzi, W. Gawelda, A. Galler, C. Bressler, G. Doumy, A. M. March, E. P. Kanter, L. Young, S. H. Southworth, S. E. Canton, J. Uhlig, G. Smolentsev, V. Sundstrm, K. Haldrup, T. B. van Driel, M. M. Nielsen, K. S. Kjaer, and H. T. Lemke, Journal of Electron Spectroscopy and Related Phenomena Progress in Resonant Inelastic X-Ray Scattering, **188**, 166 (2013).

[6] G. Peng, F. M. F. deGroot, K. Haemaelaeinen, J. A. Moore, X. Wang, M. M. Grush, J. B.

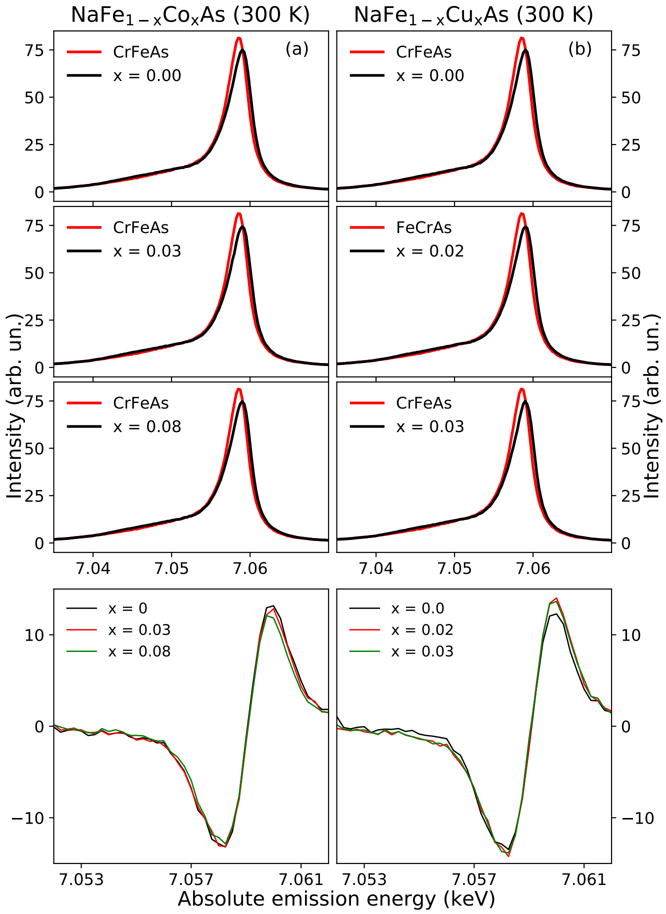


FIG. 2. (a) $K_\beta$ XES for $NaFe_{1-x}Co_xAs$ with x = 0, 0.03, and 0.08 at 300 K and spectrum of FeCrAs used for calculating the difference. (b) $K_\beta$ XES for $NaFe_{1-x}Cu_xAs$ with x = 0, 0.02, and 0.03 at 300 K and spectrum of FeCrAs used for calculating the difference. The last row is indicating the relative difference spectra for $NaFe_{1-x}Co_xAs$ and $NaFe_{1-x}Cu_xAs$ using as reference FeCrAs.

Hastings, D. P. Siddons, and W. H. Armstrong, Journal of the American Chemical Society **116**, 2914 (1994).

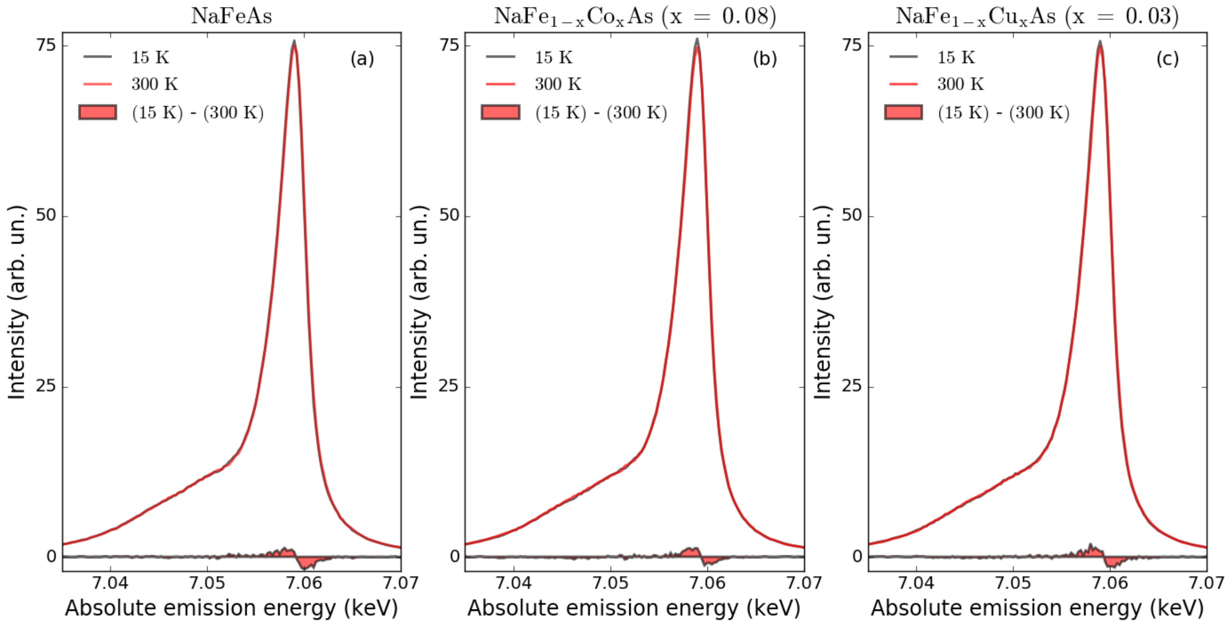


FIG. 3. Difference between XES spectra at 15 and 300 K of NaFeAs (a), $NaFe_{1-x}Co_xAs$ x = 0.08 (b) and $NaFe_{1-x}Cu_xAs$ x = 0.03 (c), respectively.
